# Supplementary material for: Double-Weighting for Covariate Shift Adaptation
Source: arXiv:2305.08637 source file (2023-06-09)
Supplement: Supplementary file 1 [file Appendix6_Multiple_Lambda.tex]

\begin{table*}[ht]
\scriptsize
\centering
\caption{Test results of real data experiments on 6 datasets in terms of classification error $\pm$ standard deviation.
The results are averages over 100 trials. $\lambda=0.001$}
\begin{tabular}{|c|c|c|c|c|c|}
\hline 
Dataset & Reweighted Exact Prob. & Robust Exact Prob. & Reweighted Estimated Prob. & Robust Estimated Prob. & KMM\\ 
\hline 
Adult & $0.31\pm0.16$ & $0.35\pm0.14$ & $0.34\pm0.17$ & $0.34\pm0.13$ & $0.29\pm0.17$ \\ 
 & $0.27\pm0.04$ & $0.26\pm0.04$ & $0.28\pm0.05$ & $0.28\pm0.04$ & $0.28\pm0.05$ \\ 
 & $0.23\pm0.07$ & $0.23\pm0.09$ & $0.26\pm0.1$ & $0.26\pm0.07$ & $0.25\pm0.09$ \\ 
\hline 
Blood & $0.36\pm0.15$ & $0.46\pm0.09$ & $0.53\pm0.12$ & $0.62\pm0.09$ & $0.34\pm0.12$ \\ 
 & $0.26\pm0.05$ & $0.27\pm0.05$ & $0.33\pm0.1$ & $0.27\pm0.04$ & $0.26\pm0.05$ \\ 
 & $0.31\pm0.1$ & $0.35\pm0.06$ & $0.45\pm0.14$ & $0.36\pm0.07$ & $0.3\pm0.07$ \\ 
\hline 
Diabetes & $0.27\pm0.15$ & $0.32\pm0.11$ & $0.35\pm0.11$ & $0.28\pm0.15$ & $0.33\pm0.16$ \\ 
 & $0.14\pm0.04$ & $0.14\pm0.04$ & $0.15\pm0.03$ & $0.14\pm0.04$ & $0.14\pm0.04$ \\ 
 & $0.17\pm0.08$ & $0.18\pm0.07$ & $0.21\pm0.06$ & $0.18\pm0.07$ & $0.18\pm0.08$ \\ 
\hline 
Haberman & $0.37\pm0.18$ & $0.32\pm0.11$ & $0.38\pm0.15$ & $0.59\pm0.13$ & $0.37\pm0.18$ \\ 
 & $0.26\pm0.06$ & $0.25\pm0.07$ & $0.32\pm0.1$ & $0.31\pm0.08$ & $0.28\pm0.08$ \\ 
 & $0.29\pm0.09$ & $0.3\pm0.09$ & $0.4\pm0.12$ & $0.45\pm0.11$ & $0.3\pm0.11$ \\ 
\hline 
Heart & $0.3\pm0.19$ & $0.35\pm0.25$ & $0.28\pm0.17$ & $0.2\pm0.13$ & $0.54\pm0.22$ \\ 
 & $0.1\pm0.04$ & $0.1\pm0.04$ & $0.11\pm0.05$ & $0.11\pm0.05$ & $0.09\pm0.04$ \\ 
 & $0.13\pm0.09$ & $0.13\pm0.06$ & $0.16\pm0.1$ & $0.16\pm0.09$ & $0.17\pm0.11$ \\ 
\hline 
Magic & $0.23\pm0.07$ & $0.3\pm0.09$ & $0.44\pm0.18$ & $0.52\pm0.18$ & $0.26\pm0.09$ \\ 
 & $0.18\pm0.02$ & $0.19\pm0.02$ & $0.19\pm0.02$ & $0.19\pm0.02$ & $0.19\pm0.02$ \\ 
 & $0.19\pm0.02$ & $0.2\pm0.02$ & $0.21\pm0.02$ & $0.21\pm0.02$ & $0.19\pm0.02$ \\ 
\hline
\end{tabular}
\label{TableL1:Experiment_Lambda_1}
\end{table*}
%%%%%%%%%%%%%%%%%%%%%%%%%%%%%%%%%%%%%%%%%%%
\begin{table*}[ht]
\scriptsize
\centering
\caption{Test results of real data experiments on 6 datasets in terms of classification error $\pm$ standard deviation.
The results are averages over 100 trials. $\lambda=0.01$}
\begin{tabular}{|c|c|c|c|c|c|}
\hline 
Dataset & Reweighted Exact Prob. & Robust Exact Prob. & Reweighted Estimated Prob. & Robust Estimated Prob. & KMM\\ 
\hline 
Adult & $0.32\pm0.16$ & $0.35\pm0.14$ & $0.34\pm0.18$ & $0.35\pm0.13$ & $0.29\pm0.17$ \\ 
 & $0.27\pm0.04$ & $0.27\pm0.04$ & $0.28\pm0.05$ & $0.28\pm0.04$ & $0.28\pm0.05$ \\ 
 & $0.23\pm0.07$ & $0.23\pm0.09$ & $0.26\pm0.1$ & $0.26\pm0.07$ & $0.25\pm0.08$ \\ 
\hline 
Blood & $0.36\pm0.15$ & $0.46\pm0.09$ & $0.53\pm0.12$ & $0.62\pm0.09$ & $0.34\pm0.12$ \\ 
 & $0.26\pm0.05$ & $0.27\pm0.05$ & $0.33\pm0.1$ & $0.27\pm0.04$ & $0.26\pm0.05$ \\ 
 & $0.31\pm0.1$ & $0.35\pm0.06$ & $0.45\pm0.14$ & $0.36\pm0.07$ & $0.3\pm0.07$ \\ 
\hline 
Diabetes & $0.27\pm0.15$ & $0.32\pm0.11$ & $0.35\pm0.11$ & $0.28\pm0.15$ & $0.33\pm0.16$ \\ 
 & $0.14\pm0.04$ & $0.14\pm0.04$ & $0.15\pm0.03$ & $0.14\pm0.04$ & $0.14\pm0.04$ \\ 
 & $0.17\pm0.08$ & $0.18\pm0.07$ & $0.21\pm0.06$ & $0.18\pm0.07$ & $0.18\pm0.08$ \\ 
\hline 
Haberman & $0.37\pm0.18$ & $0.32\pm0.11$ & $0.38\pm0.15$ & $0.59\pm0.13$ & $0.37\pm0.18$ \\ 
 & $0.26\pm0.06$ & $0.25\pm0.07$ & $0.32\pm0.1$ & $0.31\pm0.08$ & $0.28\pm0.08$ \\ 
 & $0.29\pm0.09$ & $0.3\pm0.09$ & $0.4\pm0.12$ & $0.45\pm0.11$ & $0.3\pm0.11$ \\ 
\hline 
Heart & $0.3\pm0.19$ & $0.35\pm0.25$ & $0.28\pm0.17$ & $0.2\pm0.13$ & $0.54\pm0.22$ \\ 
 & $0.1\pm0.04$ & $0.1\pm0.04$ & $0.11\pm0.05$ & $0.11\pm0.05$ & $0.09\pm0.04$ \\ 
 & $0.13\pm0.09$ & $0.13\pm0.06$ & $0.16\pm0.1$ & $0.16\pm0.09$ & $0.17\pm0.11$ \\ 
\hline 
Magic & $0.24\pm0.07$ & $0.29\pm0.09$ & $0.43\pm0.18$ & $0.51\pm0.18$ & $0.26\pm0.09$ \\ 
 & $0.18\pm0.02$ & $0.19\pm0.02$ & $0.19\pm0.02$ & $0.19\pm0.02$ & $0.19\pm0.02$ \\ 
 & $0.19\pm0.02$ & $0.2\pm0.02$ & $0.21\pm0.02$ & $0.2\pm0.02$ & $0.19\pm0.02$ \\ 
\hline
\end{tabular}
\label{TableL2:Experiment_Lambda_2}
\end{table*}
%%%%%%%%%%%%%%%%%%%%%%%%%%%%%%%%%%%%%%%%%%%%%%
\begin{table*}[ht]
\scriptsize
\centering
\caption{Test results of real data experiments on 6 datasets in terms of classification error $\pm$ standard deviation.
The results are averages over 100 trials. $\lambda=0.05$}
\begin{tabular}{|c|c|c|c|c|c|}
\hline 
Dataset & Reweighted Exact Prob. & Robust Exact Prob. & Reweighted Estimated Prob. & Robust Estimated Prob. & KMM\\
\hline 
Adult & $0.32\pm0.16$ & $0.35\pm0.14$ & $0.35\pm0.16$ & $0.35\pm0.13$ & $0.3\pm0.17$ \\ 
 & $0.27\pm0.04$ & $0.26\pm0.04$ & $0.28\pm0.05$ & $0.28\pm0.03$ & $0.28\pm0.04$ \\ 
 & $0.23\pm0.08$ & $0.23\pm0.09$ & $0.26\pm0.1$ & $0.26\pm0.08$ & $0.25\pm0.08$ \\ 
\hline 
Blood & $0.36\pm0.15$ & $0.46\pm0.09$ & $0.53\pm0.12$ & $0.62\pm0.09$ & $0.34\pm0.12$ \\ 
 & $0.26\pm0.05$ & $0.27\pm0.05$ & $0.33\pm0.1$ & $0.27\pm0.04$ & $0.26\pm0.05$ \\ 
 & $0.31\pm0.1$ & $0.35\pm0.06$ & $0.45\pm0.14$ & $0.36\pm0.07$ & $0.3\pm0.07$ \\ 
\hline 
Diabetes & $0.27\pm0.15$ & $0.32\pm0.11$ & $0.35\pm0.11$ & $0.28\pm0.15$ & $0.33\pm0.16$ \\ 
 & $0.14\pm0.04$ & $0.14\pm0.04$ & $0.15\pm0.03$ & $0.14\pm0.04$ & $0.14\pm0.04$ \\ 
 & $0.17\pm0.08$ & $0.18\pm0.07$ & $0.21\pm0.06$ & $0.18\pm0.07$ & $0.18\pm0.08$ \\ 
\hline 
Haberman & $0.37\pm0.18$ & $0.32\pm0.11$ & $0.38\pm0.15$ & $0.59\pm0.13$ & $0.37\pm0.18$ \\ 
 & $0.26\pm0.06$ & $0.25\pm0.07$ & $0.32\pm0.1$ & $0.31\pm0.08$ & $0.28\pm0.08$ \\ 
 & $0.29\pm0.09$ & $0.3\pm0.09$ & $0.4\pm0.12$ & $0.45\pm0.11$ & $0.3\pm0.11$ \\ 
\hline 
Heart & $0.3\pm0.19$ & $0.35\pm0.25$ & $0.28\pm0.17$ & $0.2\pm0.13$ & $0.54\pm0.22$ \\ 
 & $0.1\pm0.04$ & $0.1\pm0.04$ & $0.11\pm0.05$ & $0.11\pm0.05$ & $0.09\pm0.04$ \\ 
 & $0.13\pm0.08$ & $0.13\pm0.06$ & $0.16\pm0.1$ & $0.16\pm0.09$ & $0.17\pm0.12$ \\ 
\hline 
Magic & $0.23\pm0.07$ & $0.29\pm0.1$ & $0.44\pm0.19$ & $0.51\pm0.18$ & $0.26\pm0.09$ \\ 
 & $0.18\pm0.02$ & $0.18\pm0.02$ & $0.19\pm0.02$ & $0.19\pm0.02$ & $0.18\pm0.02$ \\ 
 & $0.19\pm0.02$ & $0.2\pm0.02$ & $0.21\pm0.02$ & $0.21\pm0.02$ & $0.19\pm0.02$ \\ 
\hline
\end{tabular}
\label{TableL3:Experiment_Lambda_3}
\end{table*}
%%%%%%%%%%%%%%%%%%%%%%%%%%%%%%%%%%%%
\begin{table*}[ht]
\scriptsize
\centering
\caption{Test results of real data experiments on 6 datasets in terms of classification error $\pm$ standard deviation.
The results are averages over 100 trials. $\lambda=0.1$}
\begin{tabular}{|c|c|c|c|c|c|}
\hline 
Dataset & Reweighted Exact Prob. & Robust Exact Prob. & Reweighted Estimated Prob. & Robust Estimated Prob. & KMM\\
\hline 
Adult & $0.32\pm0.16$ & $0.35\pm0.14$ & $0.35\pm0.17$ & $0.35\pm0.13$ & $0.3\pm0.16$ \\ 
 & $0.27\pm0.04$ & $0.27\pm0.04$ & $0.28\pm0.05$ & $0.28\pm0.04$ & $0.28\pm0.05$ \\ 
 & $0.23\pm0.08$ & $0.23\pm0.09$ & $0.26\pm0.1$ & $0.26\pm0.08$ & $0.25\pm0.08$ \\ 
\hline 
Blood & $0.36\pm0.15$ & $0.46\pm0.09$ & $0.53\pm0.12$ & $0.62\pm0.09$ & $0.34\pm0.12$ \\ 
 & $0.26\pm0.05$ & $0.27\pm0.05$ & $0.33\pm0.1$ & $0.27\pm0.04$ & $0.26\pm0.05$ \\ 
 & $0.31\pm0.1$ & $0.35\pm0.06$ & $0.45\pm0.14$ & $0.36\pm0.07$ & $0.3\pm0.07$ \\ 
\hline 
Diabetes & $0.27\pm0.15$ & $0.32\pm0.11$ & $0.35\pm0.11$ & $0.28\pm0.15$ & $0.33\pm0.16$ \\ 
 & $0.14\pm0.04$ & $0.14\pm0.04$ & $0.15\pm0.03$ & $0.14\pm0.04$ & $0.14\pm0.04$ \\ 
 & $0.17\pm0.08$ & $0.18\pm0.07$ & $0.21\pm0.06$ & $0.18\pm0.07$ & $0.18\pm0.08$ \\ 
\hline 
Haberman & $0.37\pm0.18$ & $0.32\pm0.11$ & $0.38\pm0.15$ & $0.59\pm0.13$ & $0.38\pm0.18$ \\ 
 & $0.26\pm0.06$ & $0.25\pm0.07$ & $0.32\pm0.1$ & $0.31\pm0.08$ & $0.28\pm0.08$ \\ 
 & $0.29\pm0.09$ & $0.3\pm0.09$ & $0.4\pm0.12$ & $0.45\pm0.11$ & $0.3\pm0.11$ \\ 
\hline 
Heart & $0.3\pm0.19$ & $0.36\pm0.25$ & $0.29\pm0.17$ & $0.21\pm0.15$ & $0.53\pm0.22$ \\ 
 & $0.1\pm0.04$ & $0.1\pm0.04$ & $0.11\pm0.05$ & $0.11\pm0.05$ & $0.09\pm0.04$ \\ 
 & $0.13\pm0.08$ & $0.13\pm0.06$ & $0.16\pm0.1$ & $0.16\pm0.09$ & $0.17\pm0.12$ \\ 
\hline 
Magic & $0.24\pm0.07$ & $0.29\pm0.09$ & $0.43\pm0.18$ & $0.51\pm0.18$ & $0.26\pm0.09$ \\ 
 & $0.18\pm0.02$ & $0.19\pm0.02$ & $0.19\pm0.02$ & $0.19\pm0.02$ & $0.19\pm0.02$ \\ 
 & $0.19\pm0.02$ & $0.2\pm0.02$ & $0.21\pm0.02$ & $0.21\pm0.02$ & $0.19\pm0.02$ \\ 
\hline
\end{tabular}
\label{TableL4:Experiment_Lambda_4}
\end{table*}
%%%%%%%%%%%%%%%%%%%%%%%%%%%%%%%%%%%%
\begin{table*}[ht]
\scriptsize
\centering
\caption{Test results of real data experiments on 6 datasets in terms of classification error $\pm$ standard deviation.
The results are averages over 100 trials. $\lambda=0.2$}
\begin{tabular}{|c|c|c|c|c|c|}
\hline 
Dataset & Reweighted Exact Prob. & Robust Exact Prob. & Reweighted Estimated Prob. & Robust Estimated Prob. & KMM\\
\hline 
Adult & $0.32\pm0.16$ & $0.35\pm0.14$ & $0.34\pm0.18$ & $0.35\pm0.13$ & $0.29\pm0.17$ \\ 
 & $0.27\pm0.04$ & $0.27\pm0.04$ & $0.28\pm0.05$ & $0.28\pm0.04$ & $0.28\pm0.05$ \\ 
 & $0.23\pm0.08$ & $0.23\pm0.09$ & $0.26\pm0.1$ & $0.26\pm0.08$ & $0.25\pm0.08$ \\ 
\hline 
Blood & $0.36\pm0.15$ & $0.46\pm0.09$ & $0.53\pm0.12$ & $0.62\pm0.09$ & $0.34\pm0.12$ \\ 
 & $0.26\pm0.05$ & $0.27\pm0.05$ & $0.33\pm0.1$ & $0.27\pm0.04$ & $0.26\pm0.05$ \\ 
 & $0.31\pm0.1$ & $0.35\pm0.06$ & $0.45\pm0.14$ & $0.36\pm0.07$ & $0.3\pm0.07$ \\ 
\hline 
Diabetes & $0.27\pm0.15$ & $0.32\pm0.11$ & $0.35\pm0.11$ & $0.28\pm0.15$ & $0.33\pm0.16$ \\ 
 & $0.14\pm0.04$ & $0.14\pm0.04$ & $0.15\pm0.03$ & $0.14\pm0.04$ & $0.14\pm0.04$ \\ 
 & $0.17\pm0.08$ & $0.18\pm0.07$ & $0.21\pm0.06$ & $0.18\pm0.07$ & $0.18\pm0.08$ \\ 
\hline 
Haberman & $0.37\pm0.18$ & $0.32\pm0.11$ & $0.38\pm0.15$ & $0.59\pm0.13$ & $0.38\pm0.18$ \\ 
 & $0.26\pm0.06$ & $0.25\pm0.07$ & $0.32\pm0.1$ & $0.31\pm0.08$ & $0.28\pm0.08$ \\ 
 & $0.29\pm0.09$ & $0.3\pm0.09$ & $0.4\pm0.12$ & $0.45\pm0.11$ & $0.3\pm0.11$ \\ 
\hline 
Heart & $0.3\pm0.19$ & $0.36\pm0.25$ & $0.29\pm0.17$ & $0.21\pm0.15$ & $0.53\pm0.22$ \\ 
 & $0.1\pm0.04$ & $0.1\pm0.04$ & $0.11\pm0.05$ & $0.11\pm0.05$ & $0.09\pm0.04$ \\ 
 & $0.13\pm0.09$ & $0.13\pm0.06$ & $0.16\pm0.1$ & $0.16\pm0.09$ & $0.17\pm0.11$ \\ 
\hline 
Magic & $0.24\pm0.07$ & $0.29\pm0.09$ & $0.43\pm0.18$ & $0.51\pm0.18$ & $0.26\pm0.09$ \\ 
 & $0.18\pm0.02$ & $0.19\pm0.02$ & $0.19\pm0.02$ & $0.19\pm0.02$ & $0.19\pm0.02$ \\ 
 & $0.19\pm0.02$ & $0.2\pm0.02$ & $0.21\pm0.02$ & $0.2\pm0.02$ & $0.19\pm0.02$ \\ 
\hline
\end{tabular}
\label{TableL5:Experiment_Lambda_5}
\end{table*}
%%%%%%%%%%%%%%%%%%%%%%%%%%%%%%%%%%%%
\begin{table*}[ht]
\scriptsize
\centering
\caption{Test results of real data experiments on 6 datasets in terms of classification error $\pm$ standard deviation.
The results are averages over 100 trials. $\lambda=0.5$}
\begin{tabular}{|c|c|c|c|c|c|}
\hline 
Dataset & Reweighted Exact Prob. & Robust Exact Prob. & Reweighted Estimated Prob. & Robust Estimated Prob. & KMM\\
\hline 
Adult & $0.31\pm0.16$ & $0.35\pm0.14$ & $0.34\pm0.17$ & $0.34\pm0.14$ & $0.29\pm0.17$ \\ 
 & $0.27\pm0.04$ & $0.27\pm0.04$ & $0.28\pm0.05$ & $0.28\pm0.04$ & $0.28\pm0.05$ \\ 
 & $0.23\pm0.08$ & $0.23\pm0.09$ & $0.26\pm0.1$ & $0.26\pm0.08$ & $0.25\pm0.08$ \\ 
\hline 
Blood & $0.36\pm0.15$ & $0.46\pm0.09$ & $0.53\pm0.12$ & $0.62\pm0.09$ & $0.34\pm0.12$ \\ 
 & $0.26\pm0.05$ & $0.27\pm0.05$ & $0.33\pm0.1$ & $0.27\pm0.04$ & $0.26\pm0.05$ \\ 
 & $0.31\pm0.1$ & $0.35\pm0.06$ & $0.45\pm0.14$ & $0.36\pm0.07$ & $0.3\pm0.07$ \\ 
\hline 
Diabetes & $0.27\pm0.15$ & $0.32\pm0.11$ & $0.35\pm0.11$ & $0.28\pm0.15$ & $0.33\pm0.16$ \\ 
 & $0.14\pm0.04$ & $0.14\pm0.04$ & $0.15\pm0.03$ & $0.14\pm0.04$ & $0.14\pm0.04$ \\ 
 & $0.17\pm0.08$ & $0.18\pm0.07$ & $0.21\pm0.06$ & $0.18\pm0.07$ & $0.18\pm0.08$ \\ 
\hline 
Haberman & $0.37\pm0.18$ & $0.32\pm0.11$ & $0.38\pm0.15$ & $0.59\pm0.13$ & $0.37\pm0.18$ \\ 
 & $0.26\pm0.06$ & $0.25\pm0.07$ & $0.32\pm0.1$ & $0.31\pm0.08$ & $0.28\pm0.08$ \\ 
 & $0.29\pm0.09$ & $0.3\pm0.09$ & $0.4\pm0.12$ & $0.45\pm0.11$ & $0.3\pm0.11$ \\ 
\hline 
Heart & $0.3\pm0.19$ & $0.36\pm0.25$ & $0.29\pm0.17$ & $0.21\pm0.15$ & $0.53\pm0.22$ \\ 
 & $0.1\pm0.04$ & $0.1\pm0.04$ & $0.11\pm0.05$ & $0.11\pm0.05$ & $0.09\pm0.04$ \\ 
 & $0.13\pm0.09$ & $0.13\pm0.06$ & $0.16\pm0.1$ & $0.16\pm0.09$ & $0.17\pm0.11$ \\ 
\hline 
Magic & $0.24\pm0.07$ & $0.29\pm0.09$ & $0.43\pm0.18$ & $0.51\pm0.18$ & $0.26\pm0.09$ \\ 
 & $0.18\pm0.02$ & $0.19\pm0.02$ & $0.19\pm0.02$ & $0.19\pm0.02$ & $0.19\pm0.02$ \\ 
 & $0.19\pm0.02$ & $0.2\pm0.02$ & $0.21\pm0.02$ & $0.21\pm0.02$ & $0.19\pm0.02$ \\ 
\hline
\end{tabular}
\label{TableL6:Experiment_Lambda_6}
\end{table*}

\begin{table*}[ht]
\scriptsize
\centering
\caption{Test results in terms of classification error obtained by DW-GCS method with 0-1-loss using multiple values of $D$. 
The $\beta(x)$ and $\alpha(x)$ functions defined in \eqref{eq_3:alphabeta_sol} have been obtained using the exact marginal probabilities.}
\begin{tabular}{|c|c|c|c|c|c|c|c|c|}
\hline 
Dataset & $D=1$ & $D=10$ & $D=50$ & $D=100$ & $D=250$ & $D=500$ & $D=750$ & $D=1000$ \\ 
\hline 
Adult & 0.31 & 0.44 & 0.49 & 0.49 & 0.48 & 0.49 & 0.46 & 0.45 \\ 
. & 0.28 & 0.27 & 0.27 & 0.27 & 0.27 & 0.27 & 0.27 & 0.27 \\ 
. & 0.25 & 0.23 & 0.23 & 0.23 & 0.22 & 0.22 & 0.22 & 0.22 \\ 
Blood & 0.34 & 0.34 & 0.33 & 0.33 & 0.33 & 0.32 & 0.33 & 0.32 \\ 
. & 0.26 & 0.26 & 0.26 & 0.26 & 0.26 & 0.26 & 0.26 & 0.26 \\ 
. & 0.32 & 0.3 & 0.29 & 0.29 & 0.29 & 0.29 & 0.3 & 0.31 \\ 
Diabetes & 0.31 & 0.3 & 0.29 & 0.28 & 0.28 & 0.28 & 0.28 & 0.28 \\ 
. & 0.14 & 0.14 & 0.14 & 0.14 & 0.14 & 0.14 & 0.14 & 0.14 \\ 
. & 0.18 & 0.17 & 0.17 & 0.17 & 0.17 & 0.17 & 0.17 & 0.17 \\ 
Haberman & 0.36 & 0.35 & 0.34 & 0.36 & 0.35 & 0.35 & 0.36 & 0.36 \\ 
. & 0.24 & 0.24 & 0.24 & 0.24 & 0.24 & 0.24 & 0.24 & 0.24 \\ 
. & 0.29 & 0.27 & 0.26 & 0.25 & 0.25 & 0.25 & 0.27 & 0.27 \\ 
Heart & 0.42 & 0.37 & 0.33 & 0.29 & 0.28 & 0.3 & 0.29 & 0.29 \\ 
. & 0.1 & 0.1 & 0.09 & 0.1 & 0.1 & 0.1 & 0.1 & 0.1 \\ 
. & 0.12 & 0.12 & 0.12 & 0.12 & 0.11 & 0.11 & 0.12 & 0.12 \\ 
Magic & 0.24 & 0.25 & 0.25 & 0.25 & 0.24 & 0.25 & 0.25 & 0.24 \\ 
. & 0.19 & 0.19 & 0.2 & 0.2 & 0.2 & 0.2 & 0.2 & 0.2 \\ 
. & 0.2 & 0.2 & 0.2 & 0.2 & 0.2 & 0.2 & 0.2 & 0.2 \\ 
\hline 
\end{tabular}
\end{table*}

\begin{table*}[ht]
\scriptsize
\centering
\caption{Test results in terms of classification error obtained by DW-GCS method with 0-1-loss using multiple values of $D$. 
The $\beta(x)$ and $\alpha(x)$ functions defined in \eqref{eq_3:alphabeta_sol} have been obtained approximating marginals using log-linear model \citep{Sugiyama2007}.}
\begin{tabular}{|c|c|c|c|c|c|c|c|c|}
\hline 
Dataset & $D=1$ & $D=10$ & $D=50$ & $D=100$ & $D=250$ & $D=500$ & $D=750$ & $D=1000$ \\ 
\hline 
Adult & 0.28 & 0.27 & 0.26 & 0.25 & 0.24 & 0.22 & 0.22 & 0.22 \\ 
. & 0.31 & 0.31 & 0.31 & 0.31 & 0.31 & 0.31 & 0.31 & 0.31 \\ 
. & 0.33 & 0.33 & 0.33 & 0.32 & 0.32 & 0.3 & 0.3 & 0.31 \\ 
Blood & 0.54 & 0.56 & 0.56 & 0.57 & 0.57 & 0.58 & 0.58 & 0.58 \\ 
. & 0.3 & 0.3 & 0.3 & 0.3 & 0.3 & 0.3 & 0.3 & 0.3 \\ 
. & 0.4 & 0.4 & 0.4 & 0.4 & 0.4 & 0.4 & 0.4 & 0.4 \\ 
Diabetes & 0.35 & 0.36 & 0.37 & 0.38 & 0.38 & 0.38 & 0.38 & 0.38 \\ 
. & 0.15 & 0.15 & 0.15 & 0.15 & 0.15 & 0.15 & 0.15 & 0.15 \\ 
. & 0.25 & 0.25 & 0.25 & 0.25 & 0.25 & 0.25 & 0.25 & 0.25 \\ 
Haberman & 0.33 & 0.33 & 0.32 & 0.33 & 0.34 & 0.34 & 0.34 & 0.34 \\ 
. & 0.25 & 0.25 & 0.25 & 0.25 & 0.25 & 0.25 & 0.25 & 0.25 \\ 
. & 0.29 & 0.29 & 0.29 & 0.29 & 0.29 & 0.29 & 0.3 & 0.29 \\ 
Heart & 0.19 & 0.12 & 0.11 & 0.11 & 0.11 & 0.13 & 0.13 & 0.13 \\ 
. & 0.18 & 0.18 & 0.18 & 0.18 & 0.18 & 0.18 & 0.18 & 0.18 \\ 
. & 0.43 & 0.43 & 0.43 & 0.43 & 0.43 & 0.42 & 0.4 & 0.4 \\ 
Magic & 0.48 & 0.49 & 0.49 & 0.5 & 0.49 & 0.49 & 0.5 & 0.5 \\ 
. & 0.2 & 0.2 & 0.2 & 0.2 & 0.2 & 0.2 & 0.2 & 0.2 \\ 
. & 0.22 & 0.22 & 0.22 & 0.22 & 0.22 & 0.22 & 0.22 & 0.22 \\ 
\hline 
\end{tabular}
\end{table*}

\begin{table*}[ht]
\scriptsize
\centering
\caption{Test results in terms of classification error obtained by DW-GCS method with log-loss using multiple values of $D$. 
The $\beta(x)$ and $\alpha(x)$ functions defined in \eqref{eq_3:alphabeta_sol} have been obtained using the exact marginal probabilities.}
\begin{tabular}{|c|c|c|c|c|c|c|c|c|}
\hline 
Dataset & $D=1$ & $D=10$ & $D=50$ & $D=100$ & $D=250$ & $D=500$ & $D=750$ & $D=1000$ \\ 
\hline 
Adult & 0.33 & 0.44 & 0.5 & 0.5 & 0.48 & 0.47 & 0.44 & 0.42 \\ 
. & 0.27 & 0.26 & 0.26 & 0.26 & 0.27 & 0.27 & 0.26 & 0.26 \\ 
. & 0.23 & 0.22 & 0.22 & 0.22 & 0.21 & 0.21 & 0.21 & 0.22 \\ 
Blood & 0.34 & 0.33 & 0.32 & 0.32 & 0.32 & 0.32 & 0.32 & 0.32 \\ 
. & 0.26 & 0.26 & 0.26 & 0.27 & 0.27 & 0.26 & 0.26 & 0.26 \\ 
. & 0.32 & 0.31 & 0.3 & 0.3 & 0.29 & 0.29 & 0.3 & 0.32 \\ 
Diabetes & 0.3 & 0.29 & 0.29 & 0.28 & 0.28 & 0.28 & 0.28 & 0.27 \\ 
. & 0.14 & 0.14 & 0.14 & 0.14 & 0.14 & 0.14 & 0.14 & 0.14 \\ 
. & 0.18 & 0.17 & 0.17 & 0.17 & 0.17 & 0.17 & 0.17 & 0.17 \\ 
Haberman & 0.36 & 0.35 & 0.34 & 0.36 & 0.36 & 0.36 & 0.36 & 0.36 \\ 
. & 0.26 & 0.24 & 0.25 & 0.25 & 0.25 & 0.25 & 0.25 & 0.25 \\ 
. & 0.3 & 0.27 & 0.26 & 0.26 & 0.26 & 0.26 & 0.27 & 0.28 \\ 
Heart & 0.41 & 0.39 & 0.33 & 0.3 & 0.28 & 0.29 & 0.29 & 0.29 \\ 
. & 0.1 & 0.1 & 0.1 & 0.1 & 0.1 & 0.1 & 0.1 & 0.1 \\ 
. & 0.12 & 0.11 & 0.11 & 0.12 & 0.11 & 0.11 & 0.11 & 0.12 \\ 
Magic & 0.24 & 0.25 & 0.25 & 0.25 & 0.24 & 0.24 & 0.24 & 0.23 \\ 
. & 0.18 & 0.18 & 0.19 & 0.19 & 0.18 & 0.18 & 0.19 & 0.19 \\ 
. & 0.19 & 0.19 & 0.19 & 0.19 & 0.19 & 0.19 & 0.2 & 0.19 \\ 
\hline 
\end{tabular}
\end{table*}

\begin{table*}[ht]
\scriptsize
\centering
\caption{Test results in terms of classification error obtained by DW-GCS method with log-loss using multiple values of $D$. 
The $\beta(x)$ and $\alpha(x)$ functions defined in \eqref{eq_3:alphabeta_sol} have been obtained approximating marginals using log-linear model \citep{Sugiyama2007}.}
\begin{tabular}{|c|c|c|c|c|c|c|c|c|}
\hline 
Dataset & $D=1$ & $D=10$ & $D=50$ & $D=100$ & $D=250$ & $D=500$ & $D=750$ & $D=1000$ \\ 
\hline 
Adult & 0.3 & 0.29 & 0.26 & 0.25 & 0.23 & 0.22 & 0.22 & 0.21 \\ 
. & 0.31 & 0.31 & 0.31 & 0.31 & 0.3 & 0.3 & 0.3 & 0.3 \\ 
. & 0.33 & 0.33 & 0.33 & 0.33 & 0.32 & 0.31 & 0.31 & 0.31 \\ 
Blood & 0.57 & 0.58 & 0.58 & 0.58 & 0.59 & 0.58 & 0.58 & 0.58 \\ 
. & 0.31 & 0.31 & 0.31 & 0.31 & 0.31 & 0.31 & 0.31 & 0.31 \\ 
. & 0.42 & 0.42 & 0.42 & 0.42 & 0.42 & 0.42 & 0.42 & 0.42 \\ 
Diabetes & 0.35 & 0.36 & 0.37 & 0.38 & 0.38 & 0.38 & 0.38 & 0.38 \\ 
. & 0.15 & 0.15 & 0.15 & 0.15 & 0.15 & 0.15 & 0.15 & 0.15 \\ 
. & 0.24 & 0.24 & 0.24 & 0.24 & 0.24 & 0.24 & 0.24 & 0.24 \\ 
Haberman & 0.33 & 0.33 & 0.33 & 0.33 & 0.33 & 0.33 & 0.33 & 0.33 \\ 
. & 0.27 & 0.27 & 0.27 & 0.27 & 0.27 & 0.27 & 0.27 & 0.27 \\ 
. & 0.32 & 0.32 & 0.32 & 0.32 & 0.32 & 0.31 & 0.31 & 0.31 \\ 
Heart & 0.11 & 0.11 & 0.11 & 0.11 & 0.12 & 0.12 & 0.13 & 0.14 \\ 
. & 0.16 & 0.16 & 0.16 & 0.16 & 0.16 & 0.16 & 0.16 & 0.16 \\ 
. & 0.36 & 0.36 & 0.36 & 0.35 & 0.35 & 0.35 & 0.35 & 0.35 \\ 
Magic & 0.46 & 0.47 & 0.47 & 0.47 & 0.47 & 0.48 & 0.48 & 0.49 \\ 
. & 0.2 & 0.2 & 0.2 & 0.2 & 0.2 & 0.2 & 0.2 & 0.2 \\ 
. & 0.22 & 0.22 & 0.22 & 0.22 & 0.22 & 0.22 & 0.22 & 0.22 \\ 
\hline 
\end{tabular}
\end{table*}
